# Supplementary material for: Variational Inference for Graph Convolutional Networks in the Absence of Graph Data and Adversarial Settings
Source: arXiv:1906.01852 source file (2020-10-21)
Supplement: Supplementary file 1 [file supp_experiments.tex]

\section{Additional results}

\subsection{Smooth parameterization}
\label{sec:smooth}
\Cref{fig:smooth-param} compares a typical run of our algorithms using the free and smooth parameterizations of the posterior. We see that the optimizer struggles to find directions of improvement for the free parameterization, whereas for the smooth parameterization the \gls{NELBO} decreases steadily during optimization. This behavior was observed throughout several learning rate settings and we attribute it to the discrete combinatorial optimization nature of the \gls{NELBO} when using the free parameterization.

\begin{figure}[t]
	\centering
	\includegraphics[width=0.45\textwidth]{../figures/elbo_comparison}
	\caption{The \acrfull{NELBO} as a function of the number of epochs for the freely parameterized posterior (Free) and the smooth parameterization (Lowrank).
	\label{fig:smooth-param}}
\end{figure}

\subsection{Noiseless graphs}
\Cref{tab:noiseless-graphs} shows the results for the noisy graphs where we see that our approach performs similarly to standard \glspl{GCN}.
\input{table_noiseless_results}

\subsection{Noisy graphs}
\label{sec:supp-noisy}
Test \acrfull{MLL} results are given in \cref{fig:noisy-graphs-relaxed-mll}. 
\begin{figure}[t]
\centering
\includegraphics[width=0.45\textwidth]{../figures/citeseer_relaxed_adding_mean_test_likelihood}
\includegraphics[width=0.45\textwidth]{../figures/cora_relaxed_adding_mean_test_likelihood}
\caption{Results for noisy graphs on \citeseer (left) and \cora (right): \Acrfull{MLL} as a function of the ratio of additional fake links relative to the number of true links. 
	\acrshort{BGCNR}-$\smoothfactorone$ stands for the relaxed version of our method with smoothing factor $\smoothfactorone$.   		
	\label{fig:noisy-graphs-relaxed-mll} }
\end{figure}

\subsection{Feature-based graphs}
Following the methods of \cite{henaff2015deep}, a graph was estimated using \cora and \citeseer based on the node features. Given a training set with features and labels we train a fully connected network with $1$-hidden layer, $Q\in \{16,32\}$ neurons using standard \gls{RELU} activation and $0.5$ dropout between each layer. We then extract the first layer features $\tilde{\mbZ}_1 \in \mathbb{R}^{M \times Q}$ where $M$ includes training, validation and test sets and consider their distance, $d(i,j) = \parallel \tilde{\mbZ}_{1,i}-\tilde{\mbZ}_{1,j}\parallel^2$. The adjacency matrix, $\mbA$, was constructed by taking the $K\in\{8,16,32\}$ closest neighbors. Test \acrfull{MLL} results are given in \cref{fig:feature-graphs-relaxed-mll}. 

\begin{figure}[t]
	\centering
	\includegraphics[width=0.45\textwidth]{../figures/citeseer_supervised_graph_meantestlikelihood}
	\includegraphics[width=0.45\textwidth]{../figures/cora_supervised_graph_mean_test_likelihood}
	\caption{Results for feature-based graphs on \citeseer (left) and \cora (right): \Acrfull{MLL} as a function of $Q$-$K$ settings, where $Q$ is the number of hidden units and $K$ the number of neighbors used to construct the graph.  
		\acrshort{BGCNR}-$\smoothfactorone$ stands for the relaxed version of our method with smoothing factor $\smoothfactorone$. 
		\label{fig:feature-graphs-relaxed-mll}}
\end{figure}

\input{twitter}

%\subsection{Discrete posterior}
%Include all the results for the discrete posterior here
